# Supplementary material for: DARE: Diverse Visual Question Answering with Robustness Evaluation
Source: arXiv:2409.18023 source file (2025-07-21)
Supplement: Supplementary file 1 [file guidelines_count.pdf]

# Question Answering with Conditional Counting

As humans, we can easily identify and filter objects in images. It is easy to count all dogs sitting on a couch or all yellow mugs. We want to create a benchmark measuring the ability of vision and language models, such as GPT-4, to perform such tasks.

## Task

You will be presented with an image. Your task is to create questions that require to count and filter the objects in the image. The questions can include:

- colours of objects
- the position of objects e.g. on the couch
- the normal usage of objects e.g. furniture intended for sitting
- grouping several objects by a hypernym e.g. all musical instruments

Make sure that the question:

- requires to apply **at least one filtering condition** to the image (e.g. which windows are open, which dogs are on the couch, ...)
- use different types of filtering conditions. Don't use colour (or any other type) in all your questions. Be creative!
- has only one correct answer

It is important that the questions are **easy to answer for a human**.

So frame the question in an unambiguous way that only allows one correct answer!

## Examples

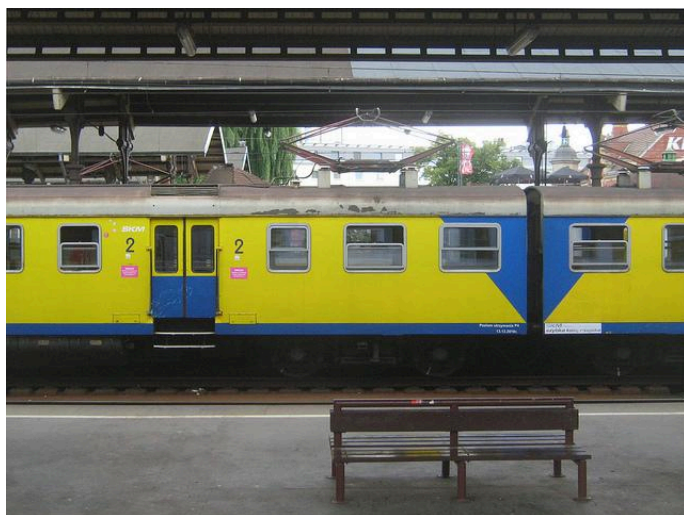

**Question:** How many windows are open?

**Correct answer:** 3

**Explanation:** The question requires not just counting all the windows, but also identifying the subset of windows that is open and counting that.

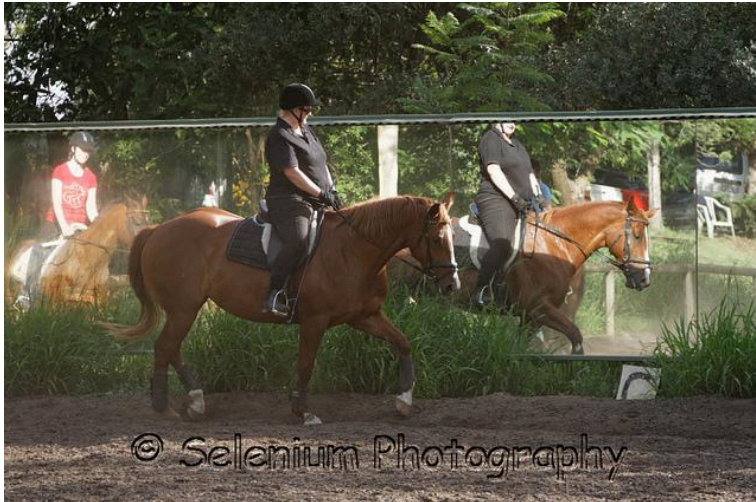

**Question:** How many horses are shown in the mirror?

**Correct answer:** 2

**Explanation:** It is not enough to count the horses in the image. Instead, the question requires the additional step to identify which horses are in the mirror.
