# Supplementary material for: DARE: Diverse Visual Question Answering with Robustness Evaluation
Source: arXiv:2409.18023 source file (2025-07-21)
Supplement: Supplementary file 2 [file guidelines_order.pdf]

# Question Answering with Ordering

To understand an image it is not enough to identify all objects within the image, but also understand where they are relative to each other (in front of, next to, in between, ....). Your task is to write questions and correct and incorrect answers for images.

## Task

For each image identify a set of objects you find interesting. Ask a question about the order, this can be the position of an object (left, centre, ...), the correct sequence of the objects, etc.

Provide **4 correct answers** that are correct and diverse. You can use:

- different words for the same thing or describe the correct order in different ways.
- different levels of object e.g. piano - music instrument, apple - fruit (but make sure the answer is unambiguous).
- different objects to describe the relative position (e.g. in between A and B, right of A, left of B, ...)

Next please provide **4 wrong answer options**. These should:

- be easy to identify as wrong to a human
- but still be plausible answers in the sense that they refer to objects in the image or objects that could be in the image
- be as likely as the correct options given only the question and not the image

Try to be as diverse and creative as you can and make them as hard as possible for a machine while the correct answers should still be easy to identify for a human.

If you can not think of an interesting question select the option that there is no interesting image and move on to the next image.

## Examples

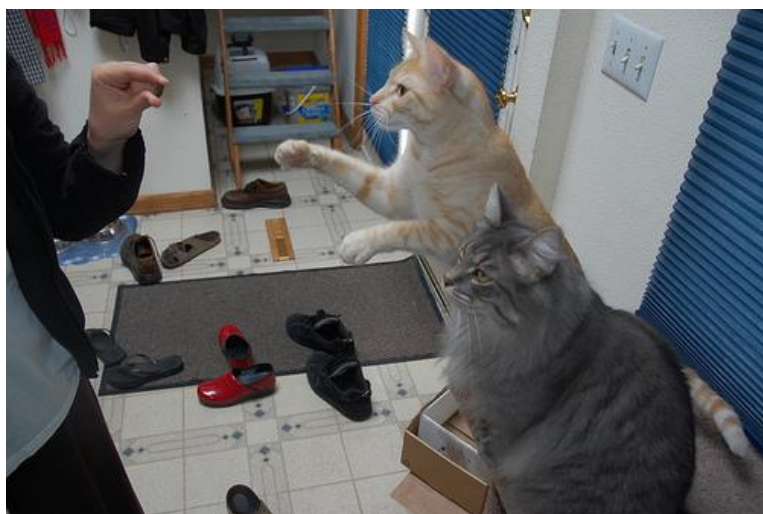

**Question:** Where are the red shoes?

**Correct answers:** in the background, partially on the carpet, behind the person and the cats, between flip-flops and black shoes

**Incorrect answers:** behind the carpet, left of the person, right of all other shoes, in the wardrobe

**Explanation:** The answers require different ways to determine the position of the shoes including background vs. foreground and being on or behind something.

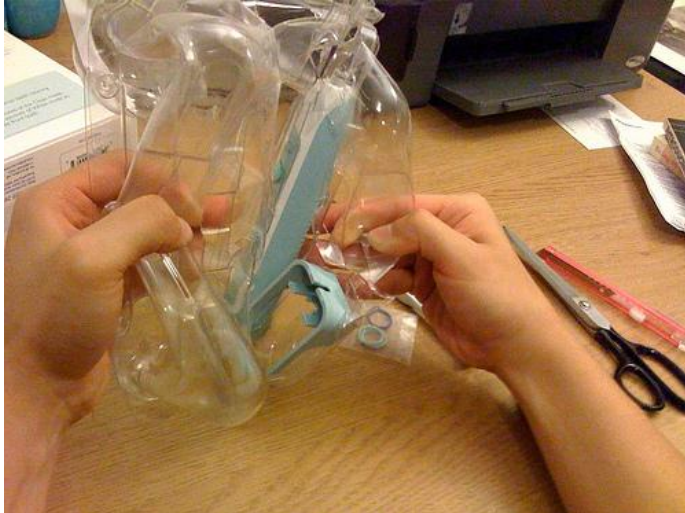

**Question:** Where are the scissors?

**Correct answer:** right of the hands, on the table, left of the cutter, next to the right hand

**Incorrect Answers:** directly next to the left hand, inside plastic packaging, on the printer, in the hand

**Explanation:** The answer options are diverse and describe the position in different ways. The wrong options are plausible e.g. scissors are often held by a hand and there is some plastic on the image that looks like packaging. It is still easy to determine between correct and incorrect answers.
